# Supplementary material for: Augmented Shuffle Differential Privacy Protocols for Large-Domain Categorical and Key-Value Data
Source: arXiv:2509.02004 source file (2025-09-02)

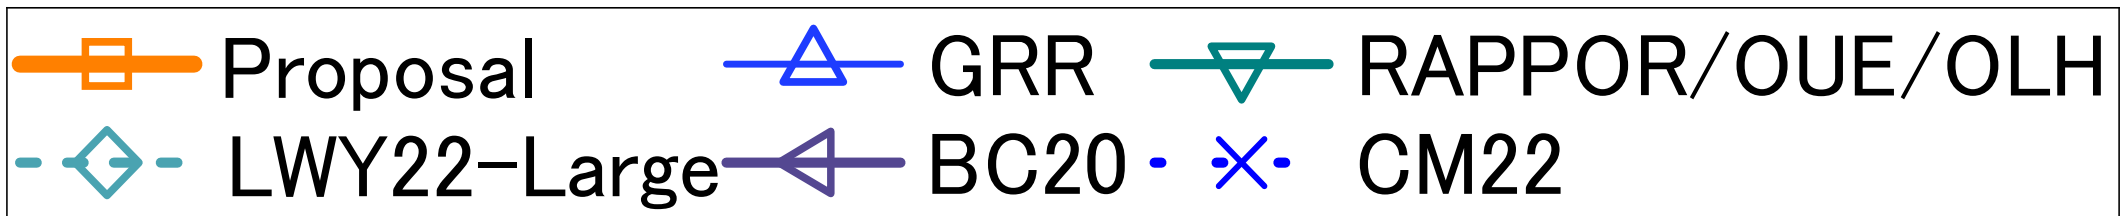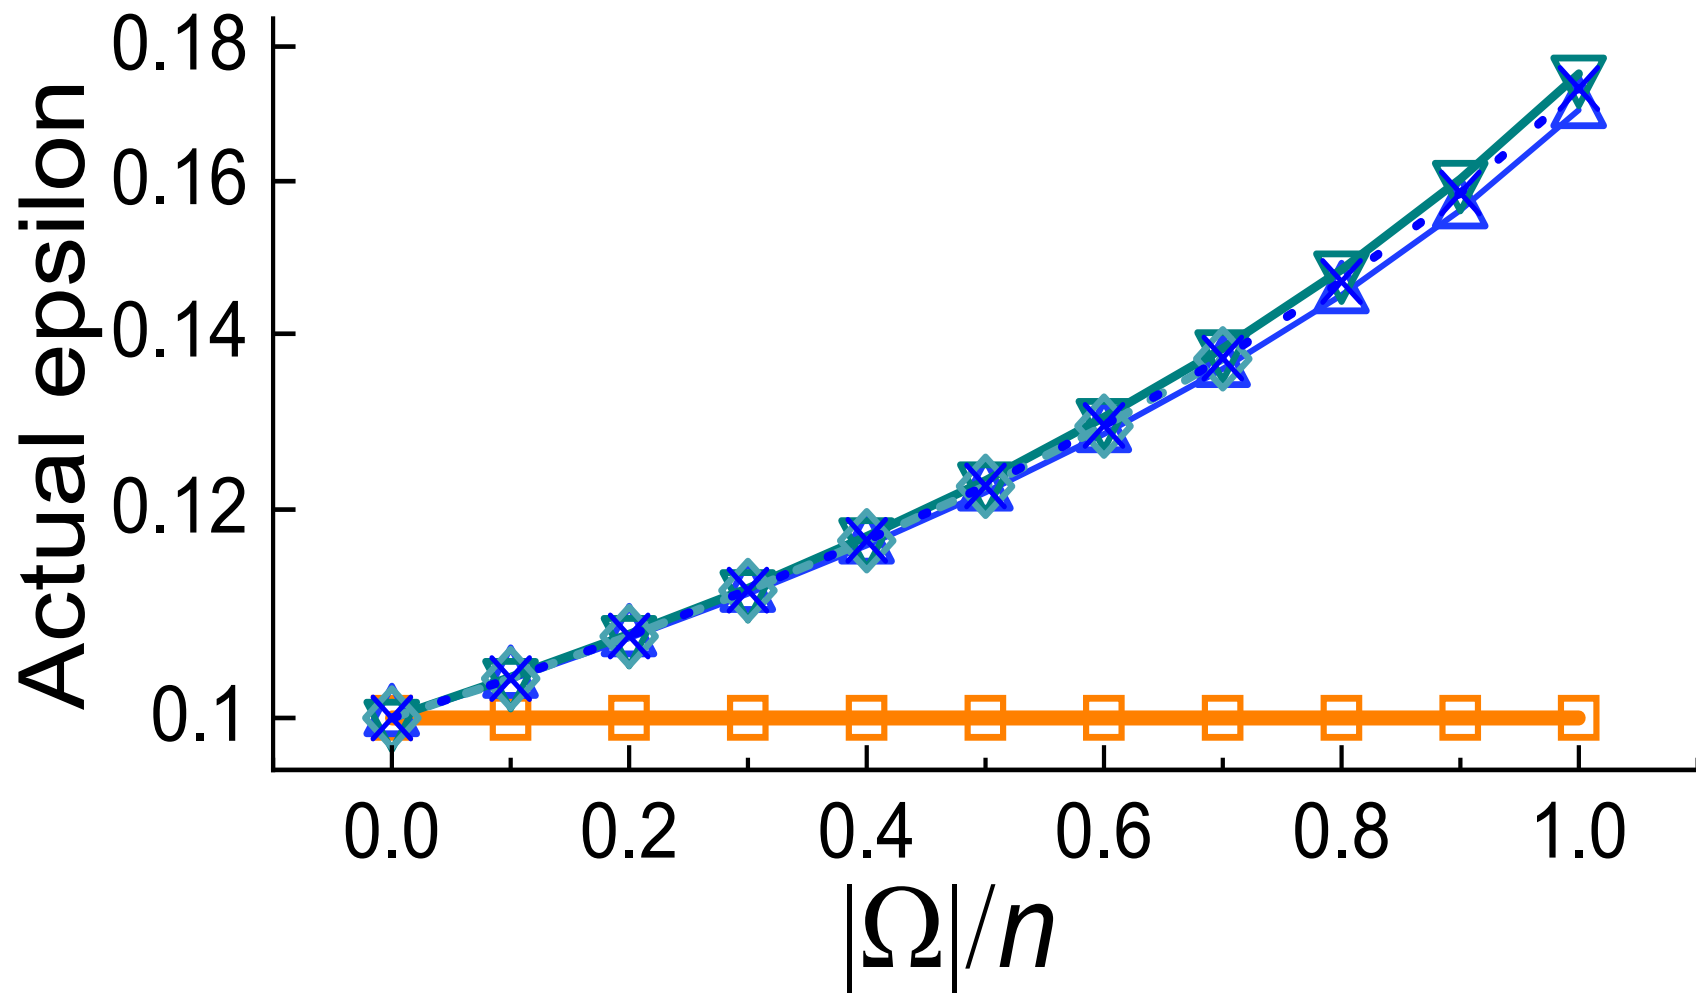

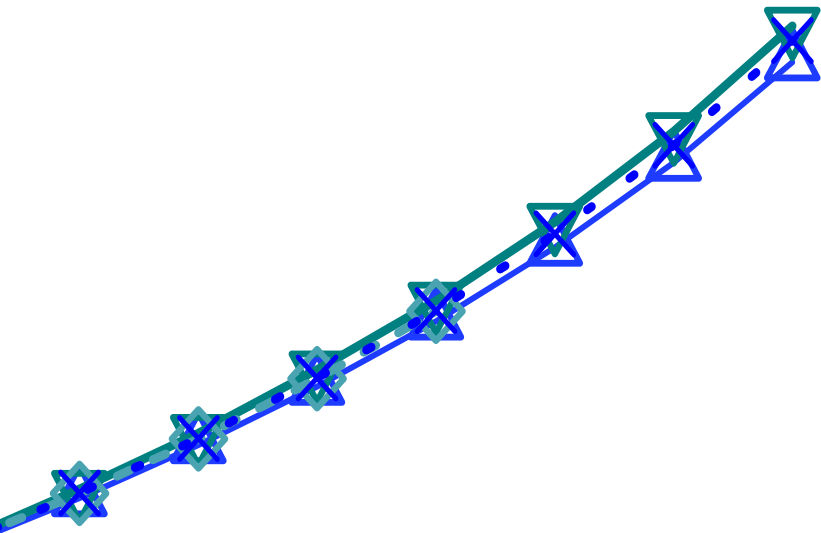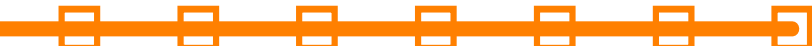

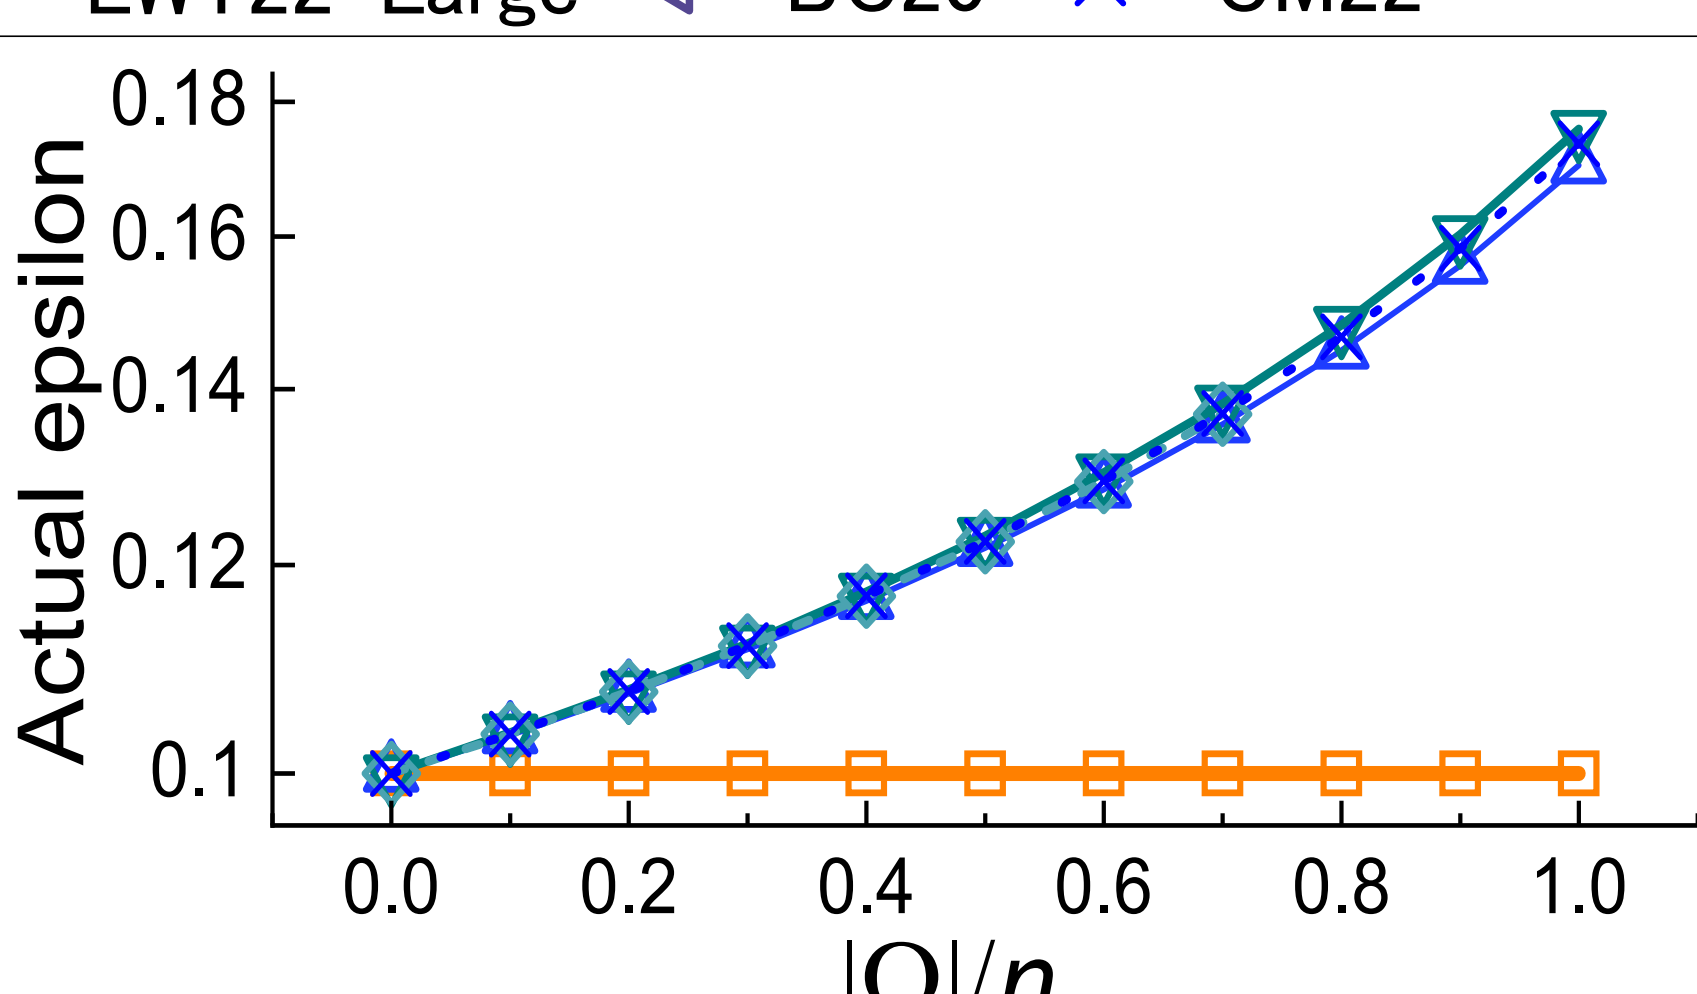

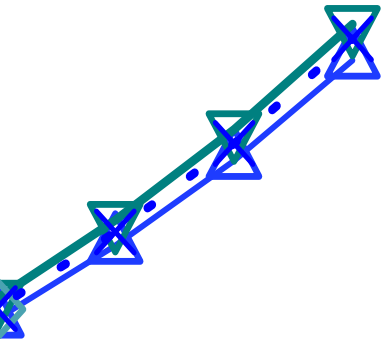

# RAPPOR/OU

## CM22

---

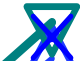

LWYZZ-Large BCZU CMZZ

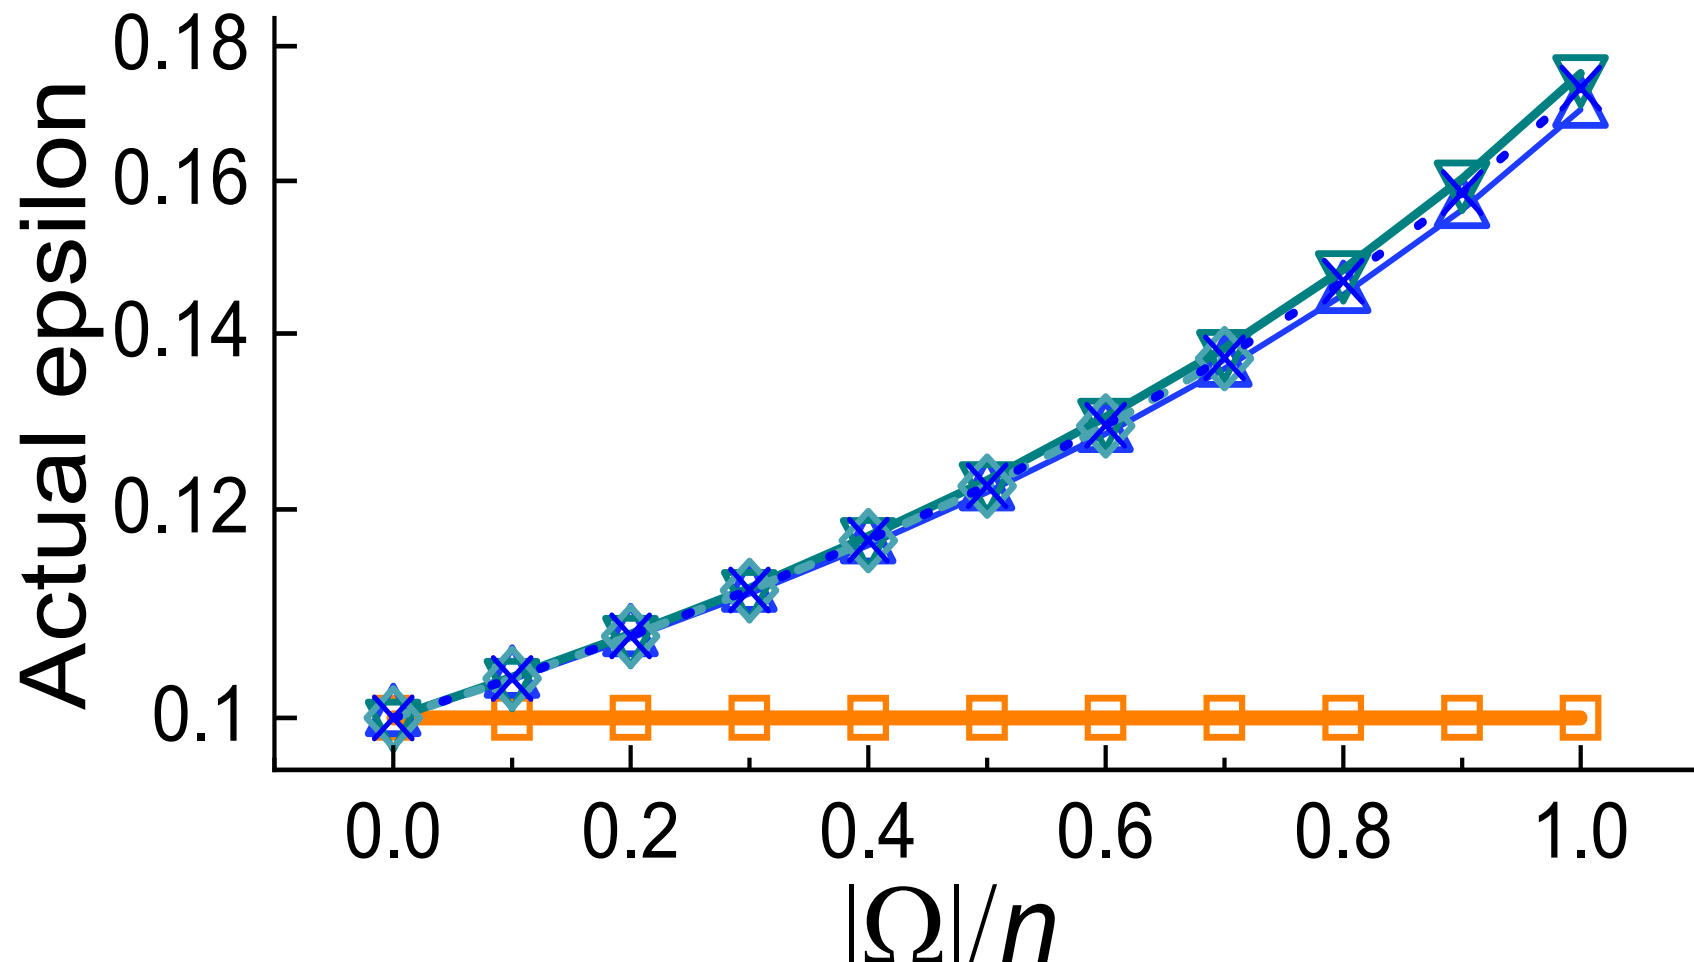

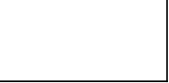

Supplement: Supplementary file 1 [file Appendix_B-A-1.pdf]
