# Supplementary material for: Augmented Shuffle Differential Privacy Protocols for Large-Domain Categorical and Key-Value Data
Source: arXiv:2509.02004 source file (2025-09-02)

Actual epsilon

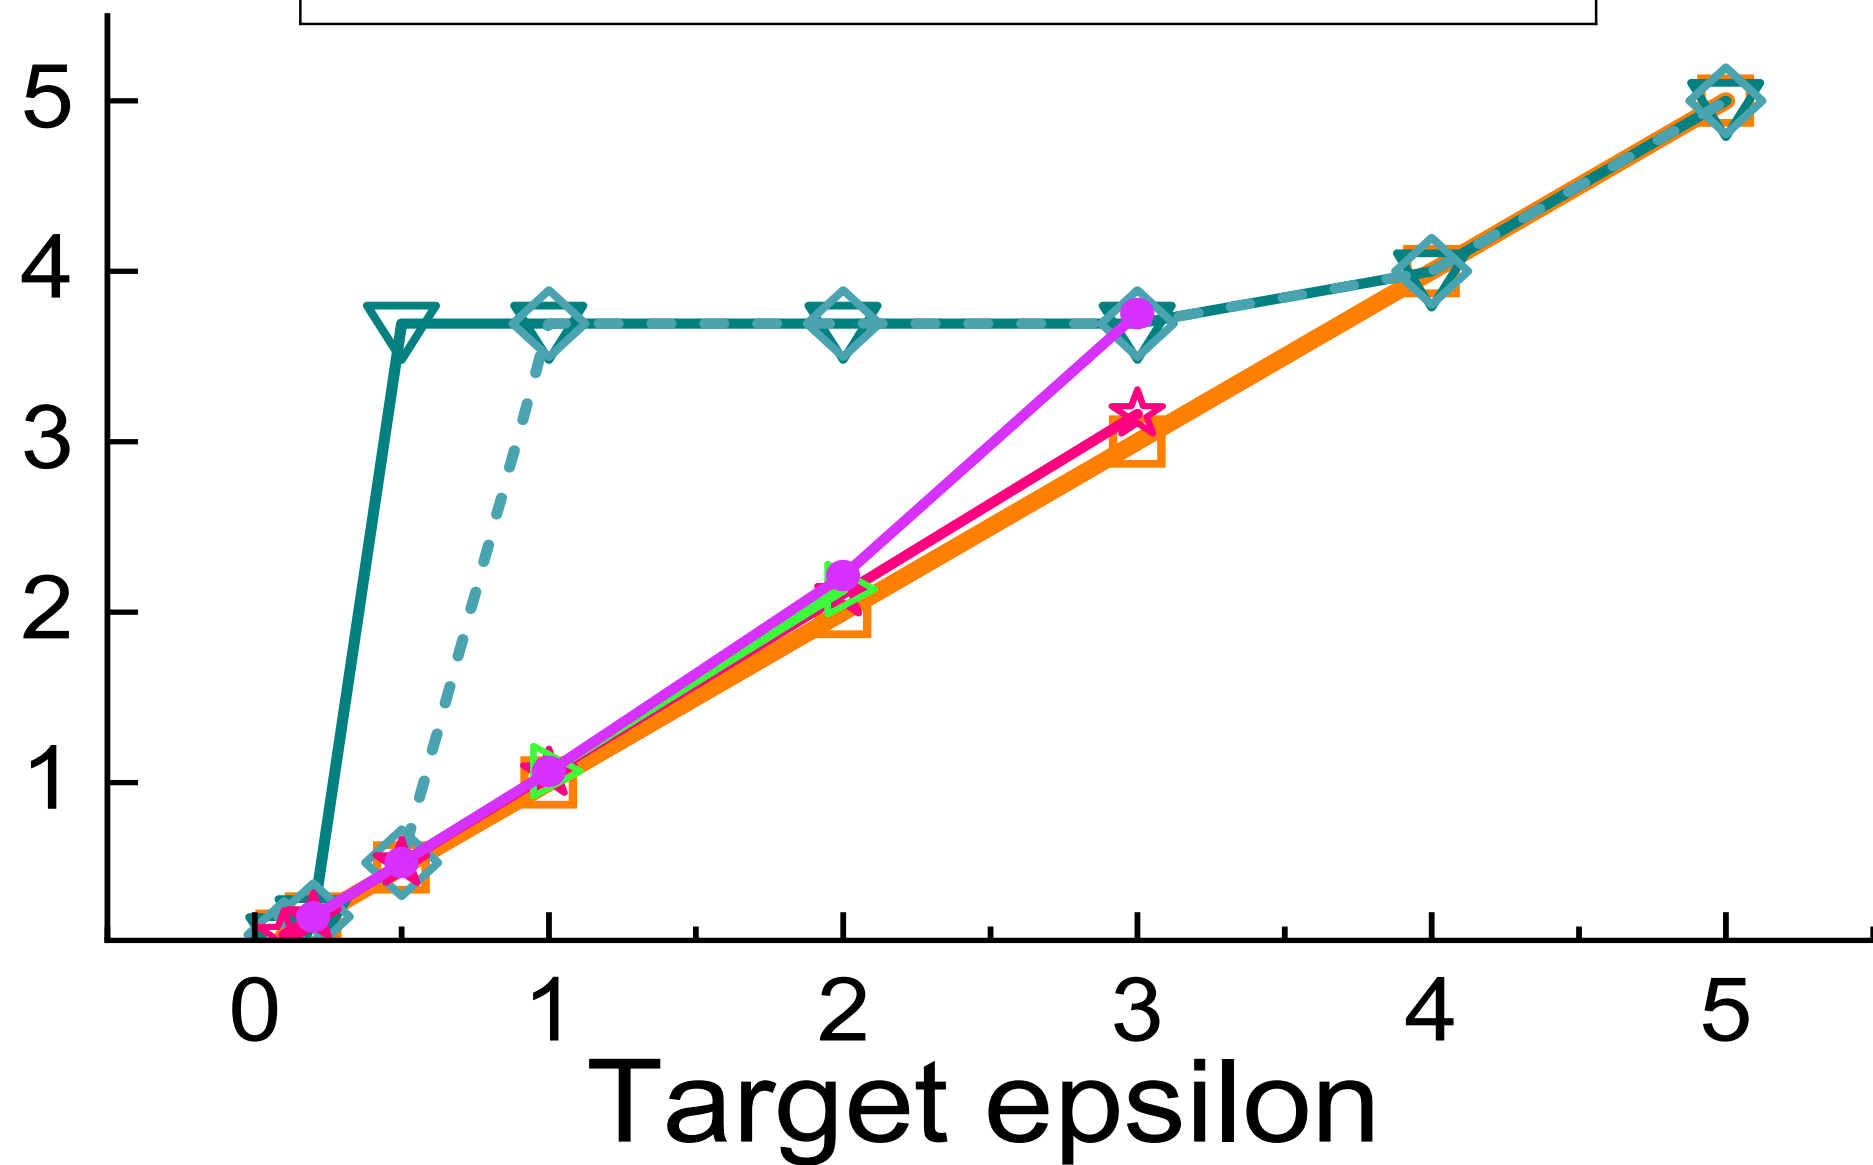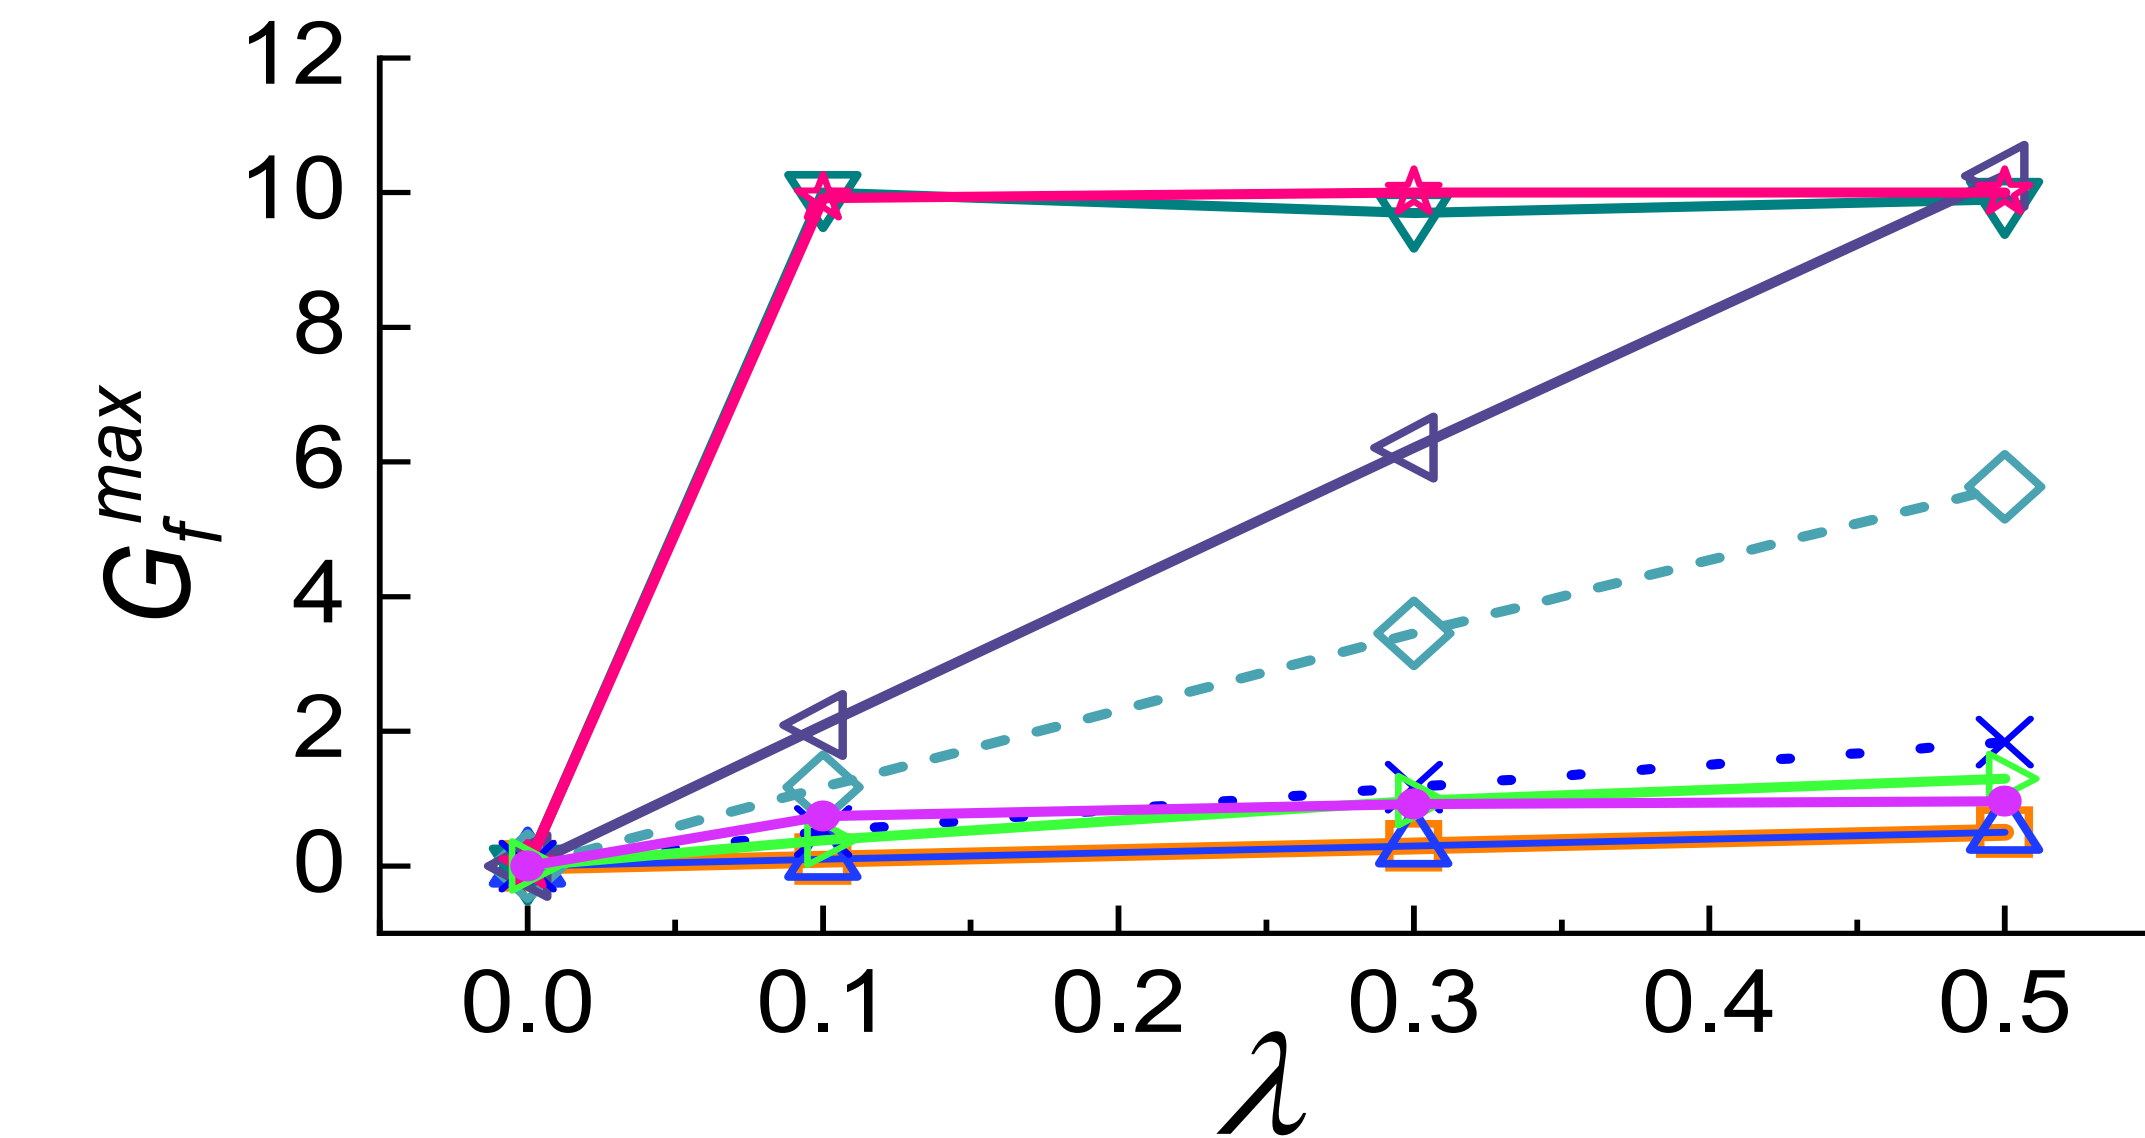

· × · OLH — ☆ —  
— ● — CM22

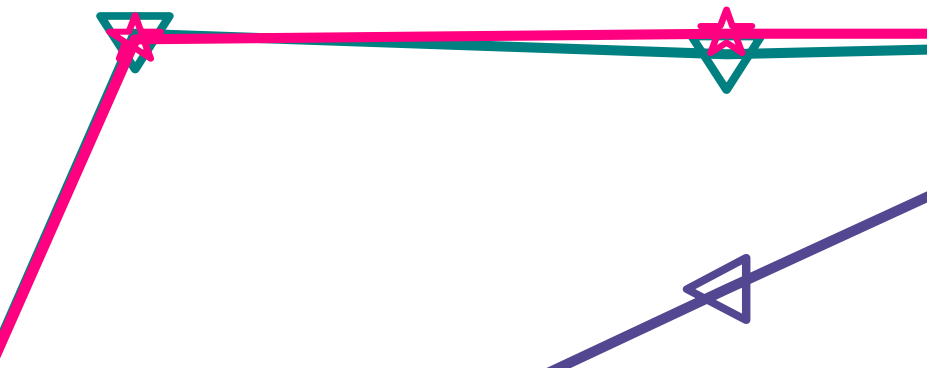

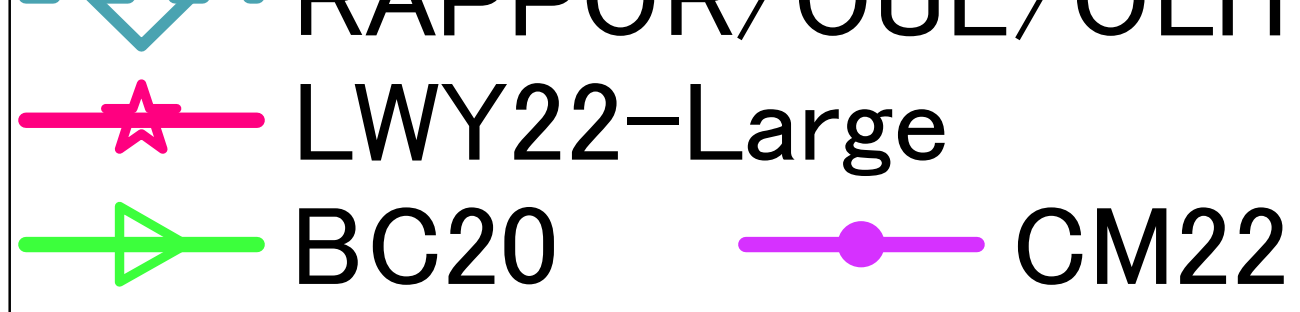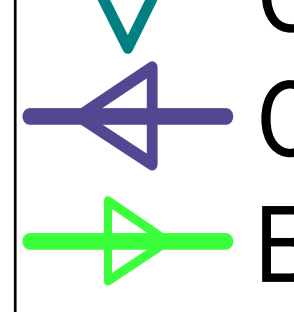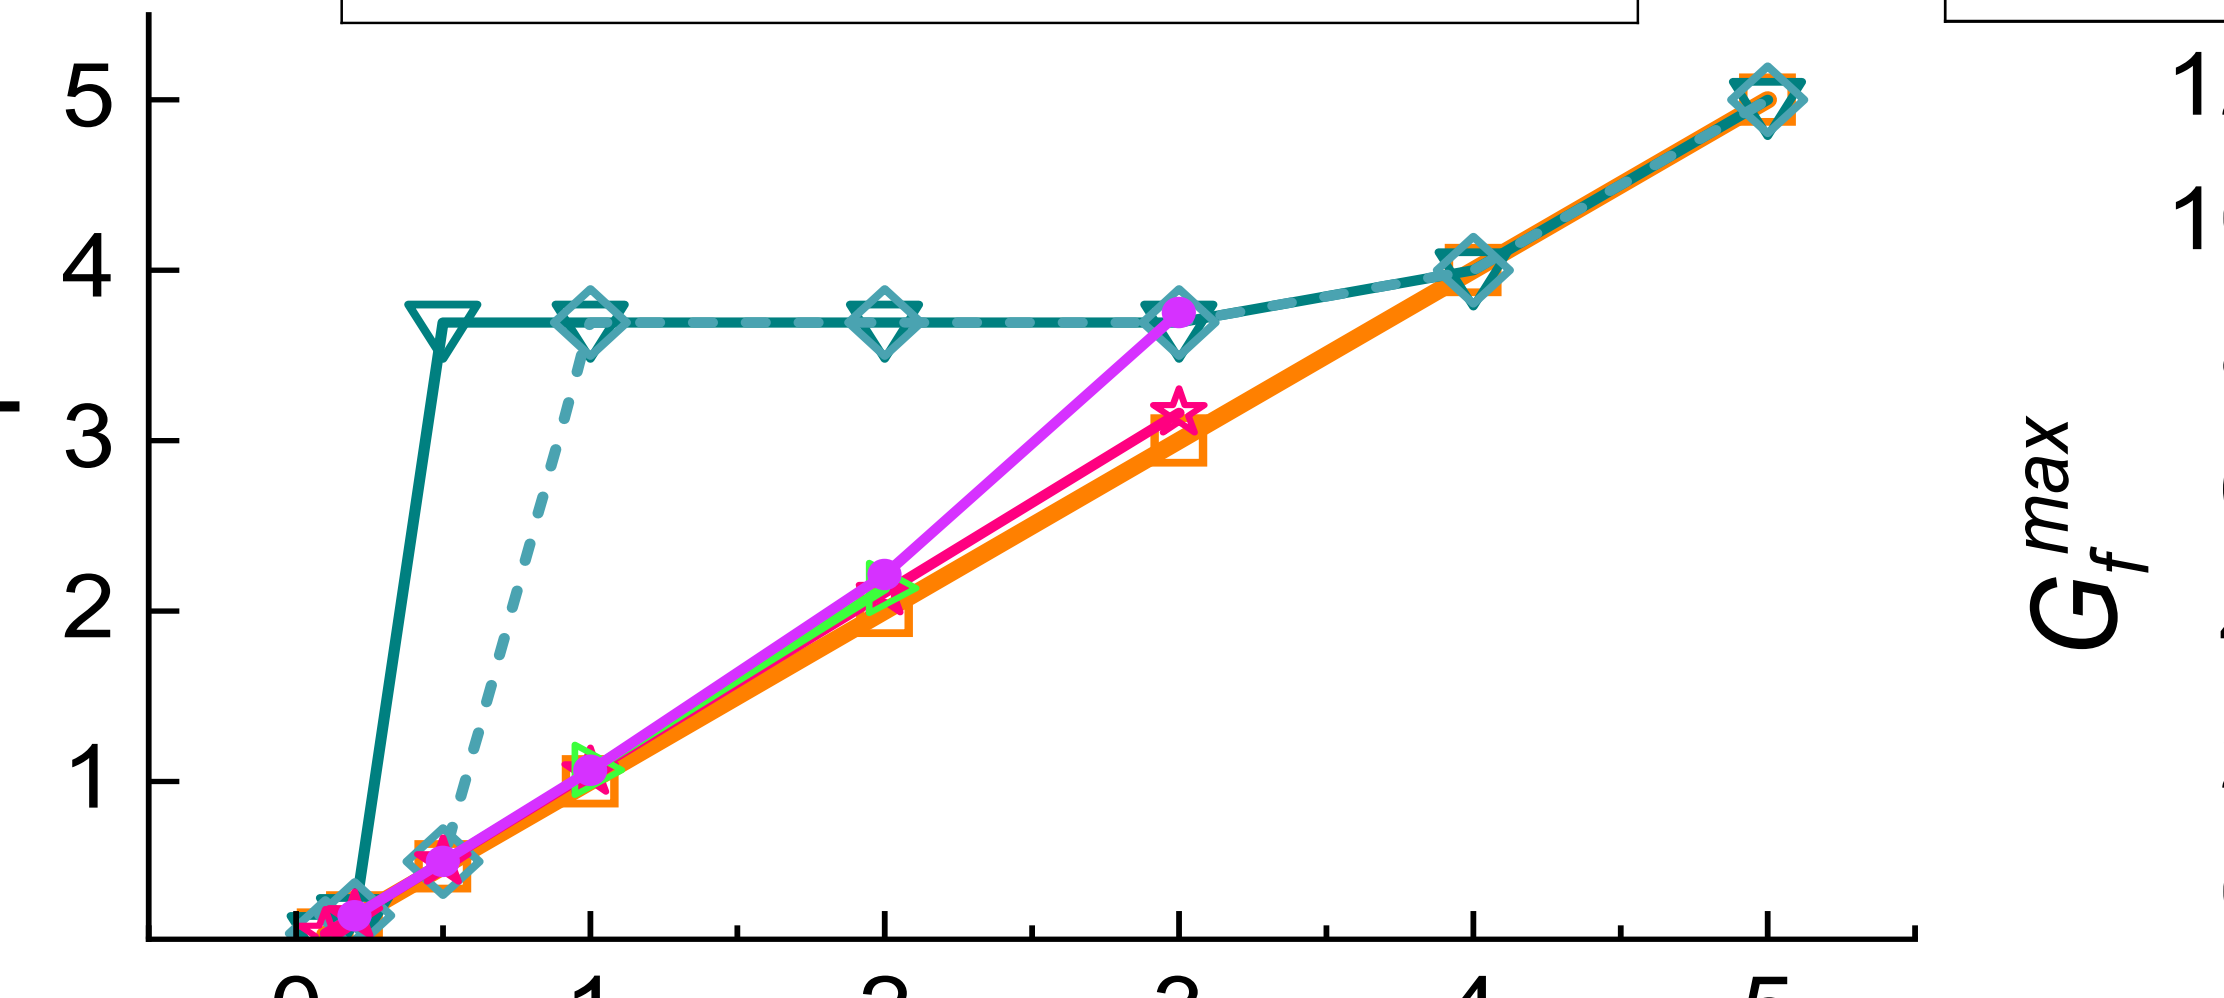

e

CM22

OUE

BC20

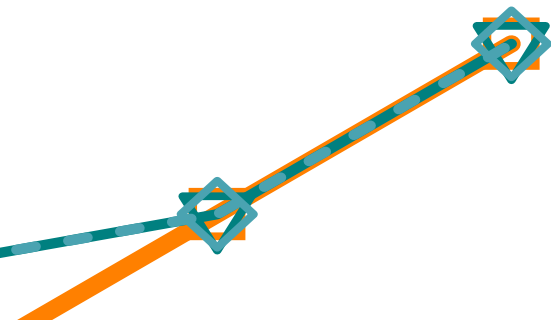

12

10

8

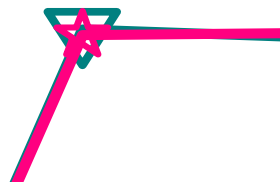

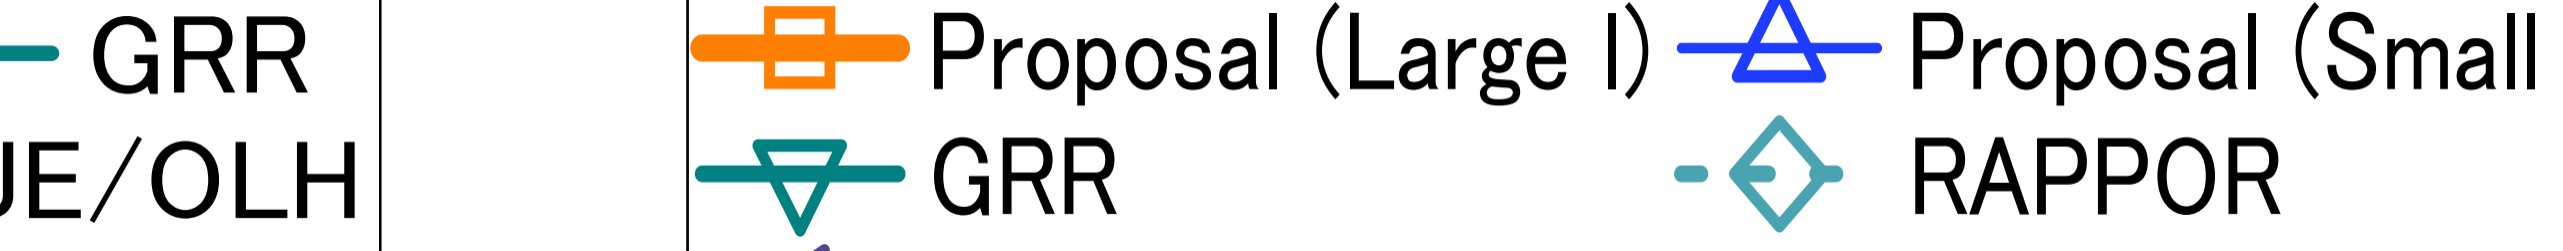

Actual options

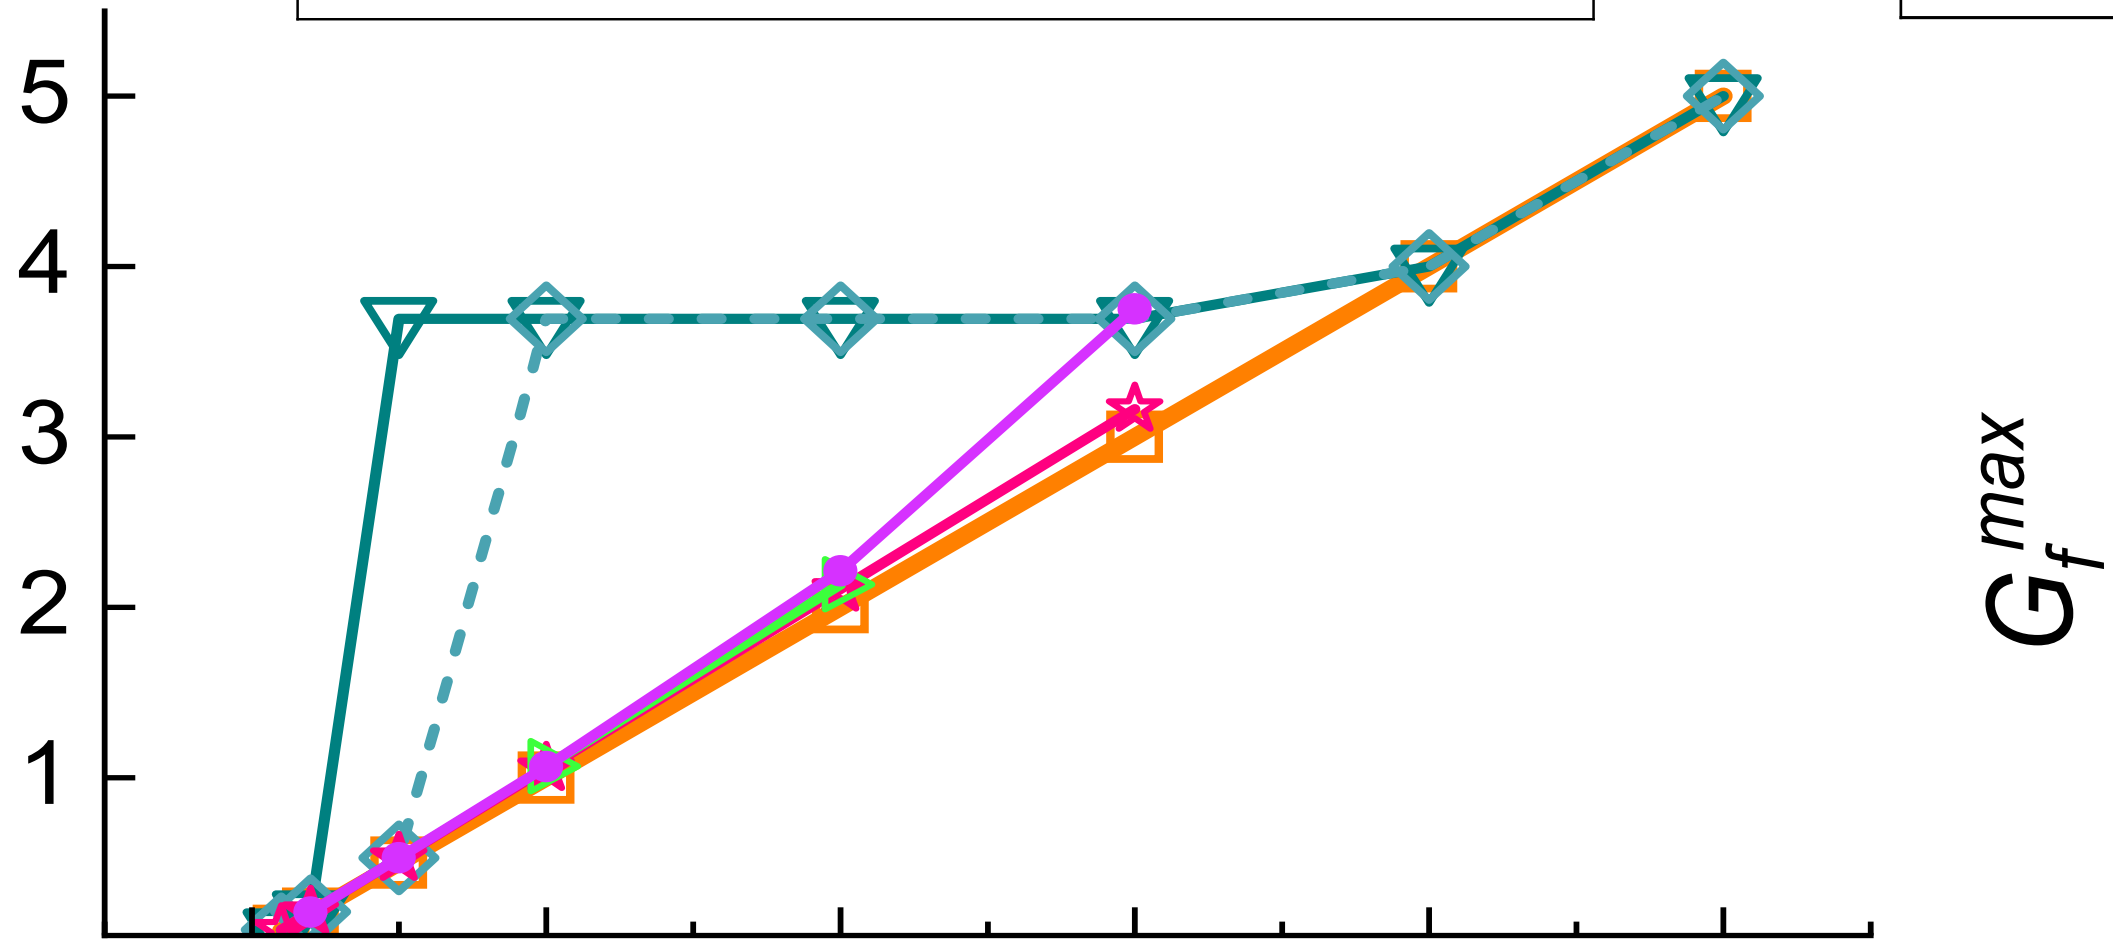

Supplement: Supplementary file 2 [file Appendix_B-C.pdf]
